# Supplementary material for: Predictability: Can the turning point and end of an expanding epidemic be precisely forecast?
Source: arXiv:2004.08842 ancillary file (2020-07-24)
Supplement: Supplementary file 1 [file SCIR-SI.pdf]

# Supplementary Information for "Predictability: Can the turning point and end of an expanding epidemic be precisely forecast while the epidemic is still spreading?"

Mario Castro, Saúl Ares, José A. Cuesta, and Susanna Manrubia

## A Analytical solution of the SCIR model at low fraction of infected individuals

If we assume that $I(t)/N \ll 1$ (consistent with the prevalence by the time of writing [1]), then we can neglect the nonlinear term in the equation for the number of susceptible individuals. Within this approximation, the equations determining the dynamics are

$$\begin{cases} \dot{S} = -qS + pC, \\ \dot{C} = qS - pC, \\ \dot{I} = \frac{\beta}{N} IS - (r+\mu)I, \\ \dot{R} = rI, \\ \dot{D} = \mu I. \end{cases} \tag{S1}$$

The first two equations imply $S + C = N$—an approximate relation consequence of our assumption $I(t) \ll N$—so we can write $C = N - S$ and reformulate the equations as

$$\begin{cases} \dot{S} = -(q+p)S + pN, \\ \dot{I} = \frac{\beta}{N} IS - (r+\mu)I. \end{cases} \tag{S2}$$

The solution of this system can be obtained in closed form as

$$S(t) = \frac{N}{q+p}\left[p + qe^{-(q+p)t}\right], \qquad R(t) = r\int_0^t I(u)\,du,$$

$$I(t) = I_0 e^{[R_0^*(t)-1](r+\mu)t} \qquad D(t) = \mu\int_0^t I(u)\,du,$$

where

$$R_0^*(t) \equiv \frac{R_0}{q+p}\left[p + q\frac{1-e^{-(q+p)t}}{(q+p)t}\right], \qquad R_0 \equiv \frac{\beta}{r+\mu}, \tag{S3}$$

is the effective basic reproduction number modulated by the confinement—$R_0$ being its value at the beginning of the epidemic.

# B Data and code

All the codes were written in the R language. The source code is publicly available as a github repository at https://github.com/mariocastro73/predictability. All the datasets have been obtained from publicly available repositories based on the official data reported by Spanish Ministry of Health and are available in `csv` format. We include here the `JAGS` code to illustrate the basic structure of the Bayesian estimation code.

```
# JAGS Code
# Regression before global confinement (populations are in log scale)
  for(t in (t0+1):(tq)) {
  I[t] ~ dnorm(I0+(beta-rmu)*(t-t0),tauI) # Active cases
  y[t] ~ dnorm(I0+(beta-rmu)*(t-t0),tauI) # Posterior predictive
  }
  # Regression for active cases post-confinement (populations are in log scale)
  for(t in (tq+1):tmax) {
  I[t] ~ dnorm(Iq+ ((beta*q)/(p+q)^2*(1-exp(-(p+q)*(t-tq)))+
       (beta-rmu-beta*q/(q+p))*(t-tq)),tauI)
  }
  # Posterior predictive for active cases post-confinement (extended until tf)
  for(t in (tq+1):tf) {
  y[t] ~ dnorm(y[tq]+
       ((beta*q)/(p+q)^2*(1-exp(-(p+q)*(t-tq)))+(beta-rmu-beta*q/(q+p))*(t-tq)),tauI)
  }
  # Regression for new deaths+recovered
  for(t in tX0:tmax) {
  X[t] ~ dnorm(log(rmu)+I[t],tauX) # New Deaths + Recovered
  }
  # Posterior predictive for new deaths+recovered (extended until tf)
  for(t in (tX0):tf) {
  z[t] ~ dnorm(log(rmu)+y[t],tauX)
  }
  # Priors for parameters
  p ~ dunif(0,5) # Non-informative prior
  q ~ dunif(0,5) # Non-informative prior
  beta ~ dunif(0,1) # Doubling time is less than 1 per day
  rmu ~ dunif(0,1) # rmu is lower than beta (so R0>1)
  # Priors for precision (inverse of variance)
  tauI ~ dgamma(0.01,0.01) # Non-informative prior
  tauX ~ dgamma(0.01,0.01)# Non-informative prior
  y[t0] <- I0
  }
```

# C Additional plots

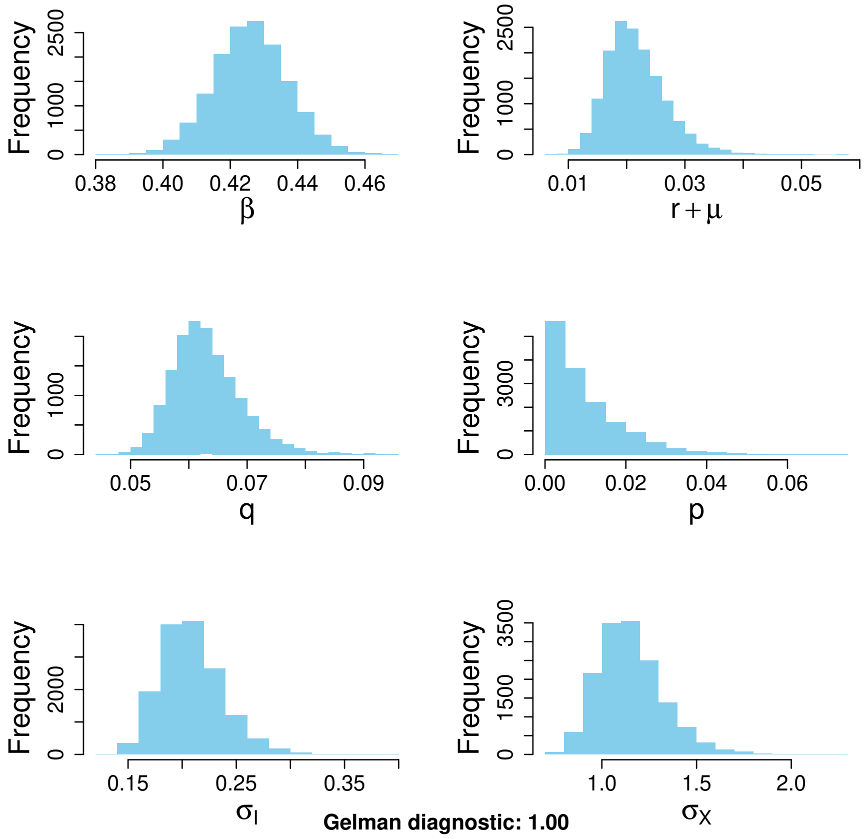


Figure S1: Parameter posteriors for the fit in Fig. 2 in the main text. The multivariate potential reduction factor is 1.00. Values close to 1 mean that different initial conditions in the Monte-Carlo Markov Chain algorithm converge with high accuracy and the fitted posteriors are reliable (see Ref. [2] for details).

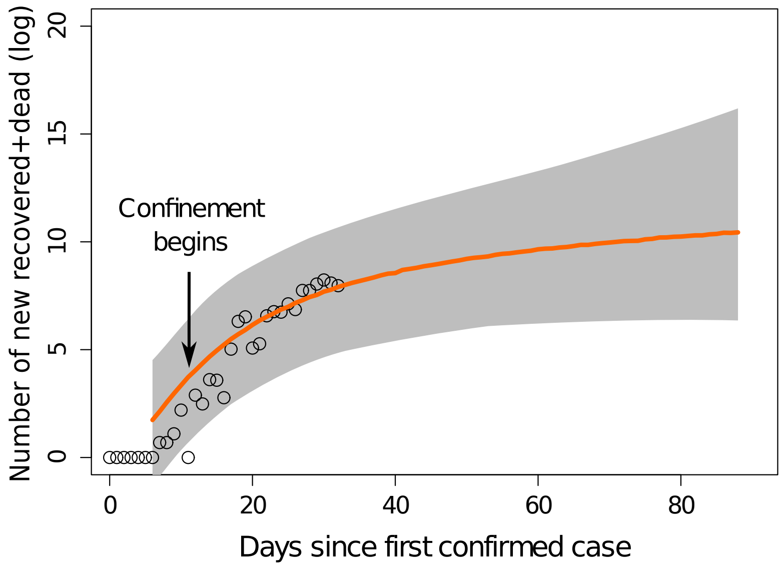


Figure S2: Fit to data for the daily number of new dead and recovered cases in Spain (from March 1st to March 29th). These data are fitted along with the number of infected cases. The fit is not as accurate as the one in Fig. 1 of the main text. This may be due to the huge variability in the latency between infection and death and recovery reported by the Spanish Ministry of Health. The shaded area represents the 95% confidence interval. As with the number of infected cases, the confidence intervals widen with time (more so taking into account that the data is represented in logarithmic scale).

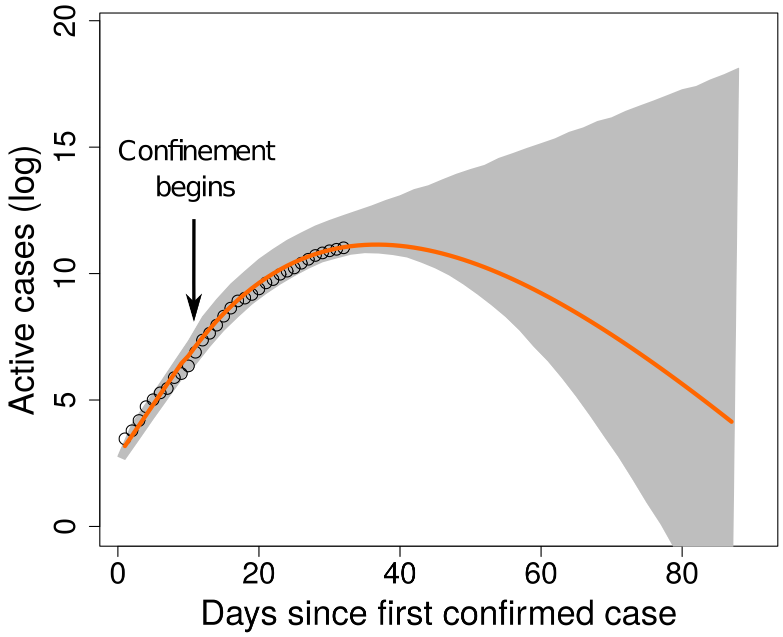


Figure S3: Impact of non-informative priors. In the description of the Bayesian model and in the main text we argued that global data analyses support that $\beta$ should be bounded by 1 day$^{-1}$. If this constraint is relaxed, we obtain the fits shown here, where we are using $\mathcal{U}(0,5)$ as priors for $\beta$ and $r+\mu$. Note how the 5%-95% quantiles are wider, so predictions are even less reliable. This points to the need of using external medical or biological data to inform the priors. Data correspond to the daily number of active cases in Spain (from March 1st to March 29th). Compare this plot to Fig. 2 in the main text.

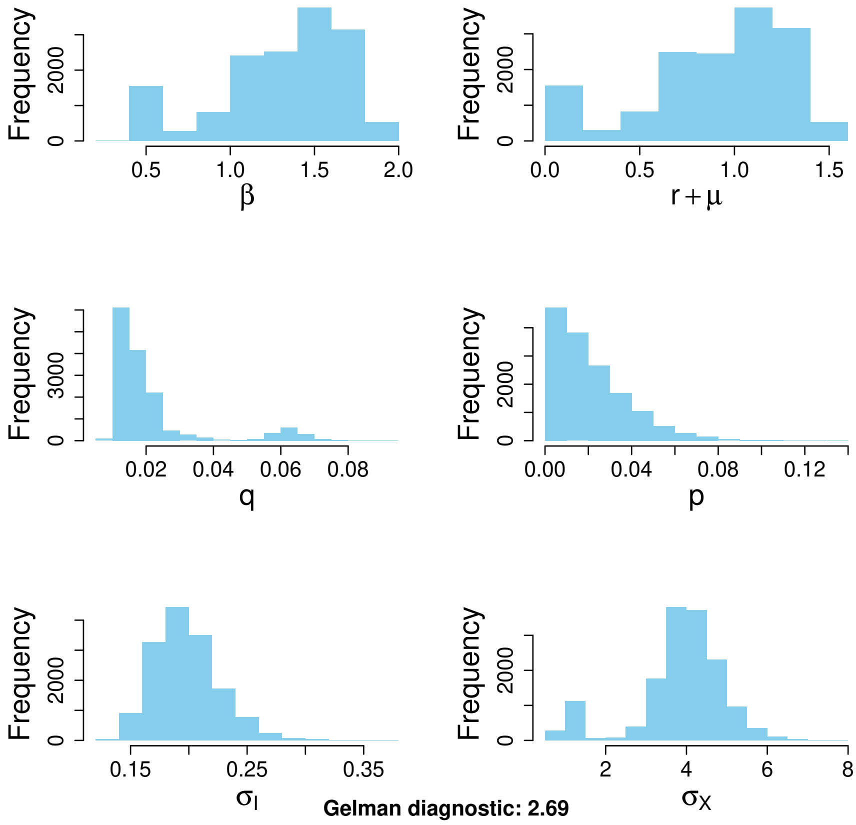


Figure S4: Posterior distributions using non-informative priors for β and $r+\mu$ (namely $\mathcal{U}(0,5)$), obtained for the fits in Fig. S3. Note that β can take values larger than 1 and that posterior distributions can be multimodal—both features indicate that the model cannot reliably determine these parameters, illustrating an identifiability problem. The multivariate potential reduction factor is now 2.69 (almost three times larger than 1, considered to be the optimal value [2]). This large value is due to the existence of different sets of parameters that can fit the data accurately.

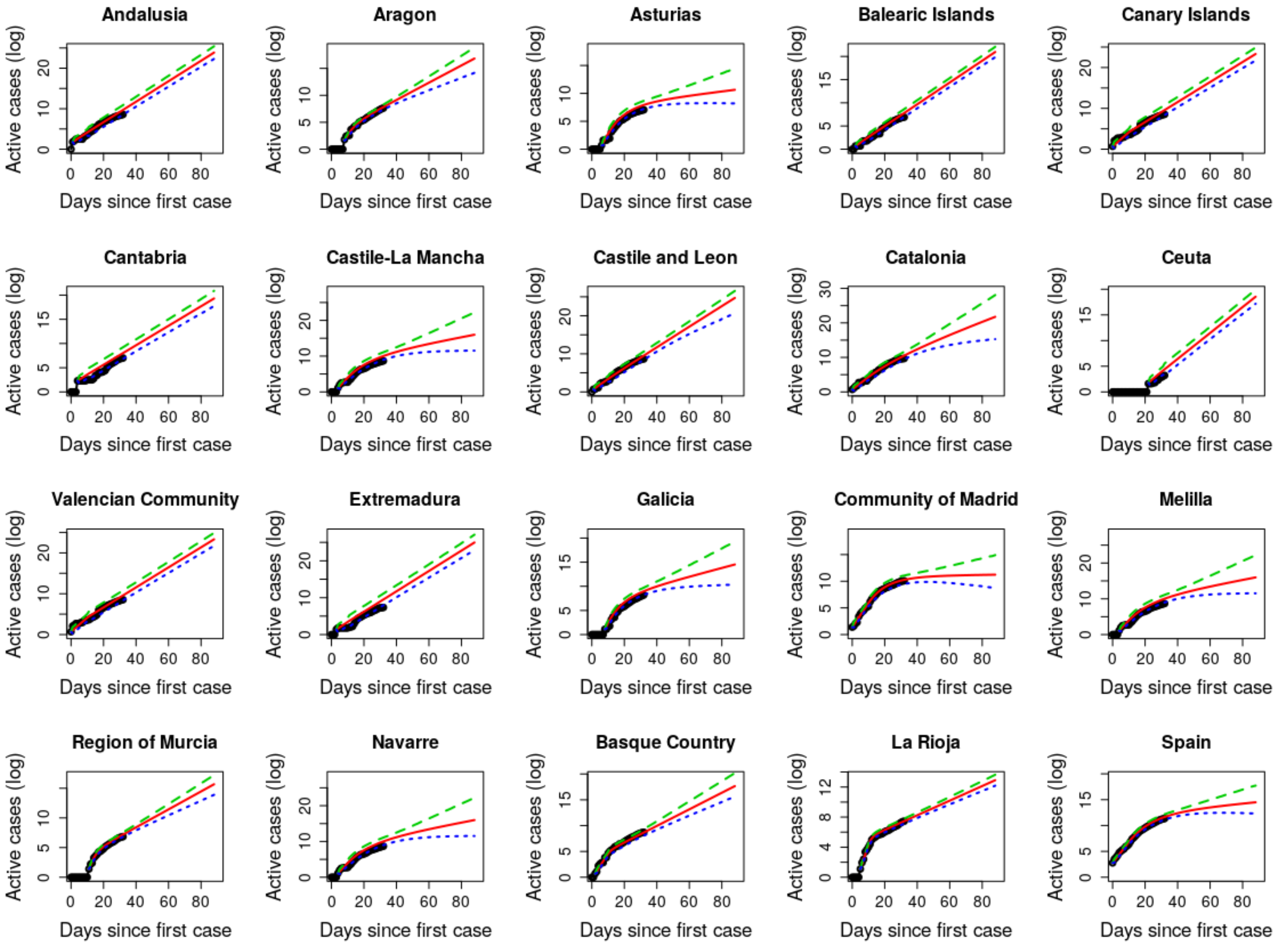


Figure S5: Model fits for every Spanish Autonomous region. Note how the aggregated data is representative only of those regions with a non-vanishing probability of decline. As in Fig. 2 in the main text, the symbols stand for the data, the solid line for the median of the posterior predictive and the colour dashed lines for the 5% and 95% percentiles.

a)

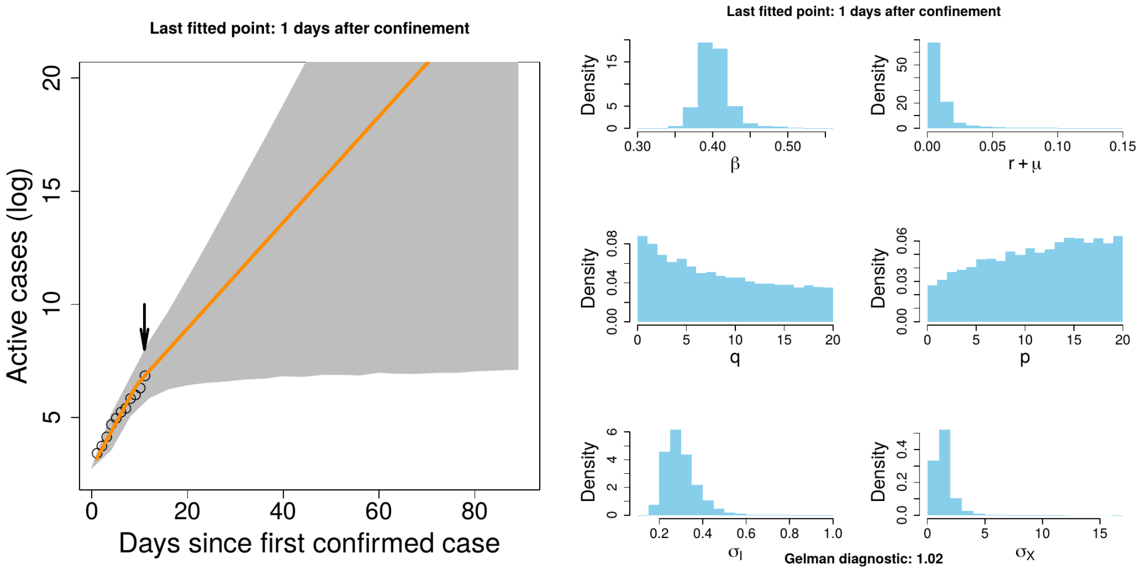


b)

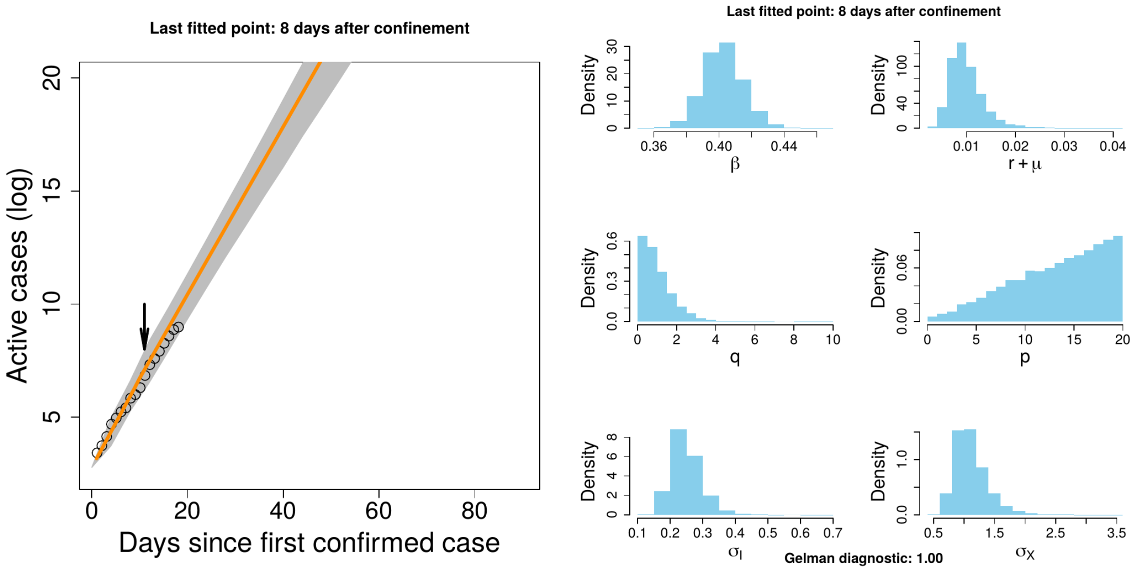


Figure S6: Median estimate with a 95% posterior predictive and posterior density using empirical data. a) Data up to 1 day after the confinement in Spain. Left: Median and 95% posterior predictive. Right: Posteriors of the parameters learnt from that data. We have used wider priors for $p$ and $q$, namely $p, q \sim \mathcal{U}(0, 20)$ to accommodate this situation. Note how the posterior for $p$ and $q$ are almost uniform meaning that we cannot learn anything about confinement so early in the epidemic. b) Panels as in a) but up to 8 days after confinement. Note how the posterior for $q$ has narrowed (meaning that confinement has started) but we still cannot infer anything about $p$.

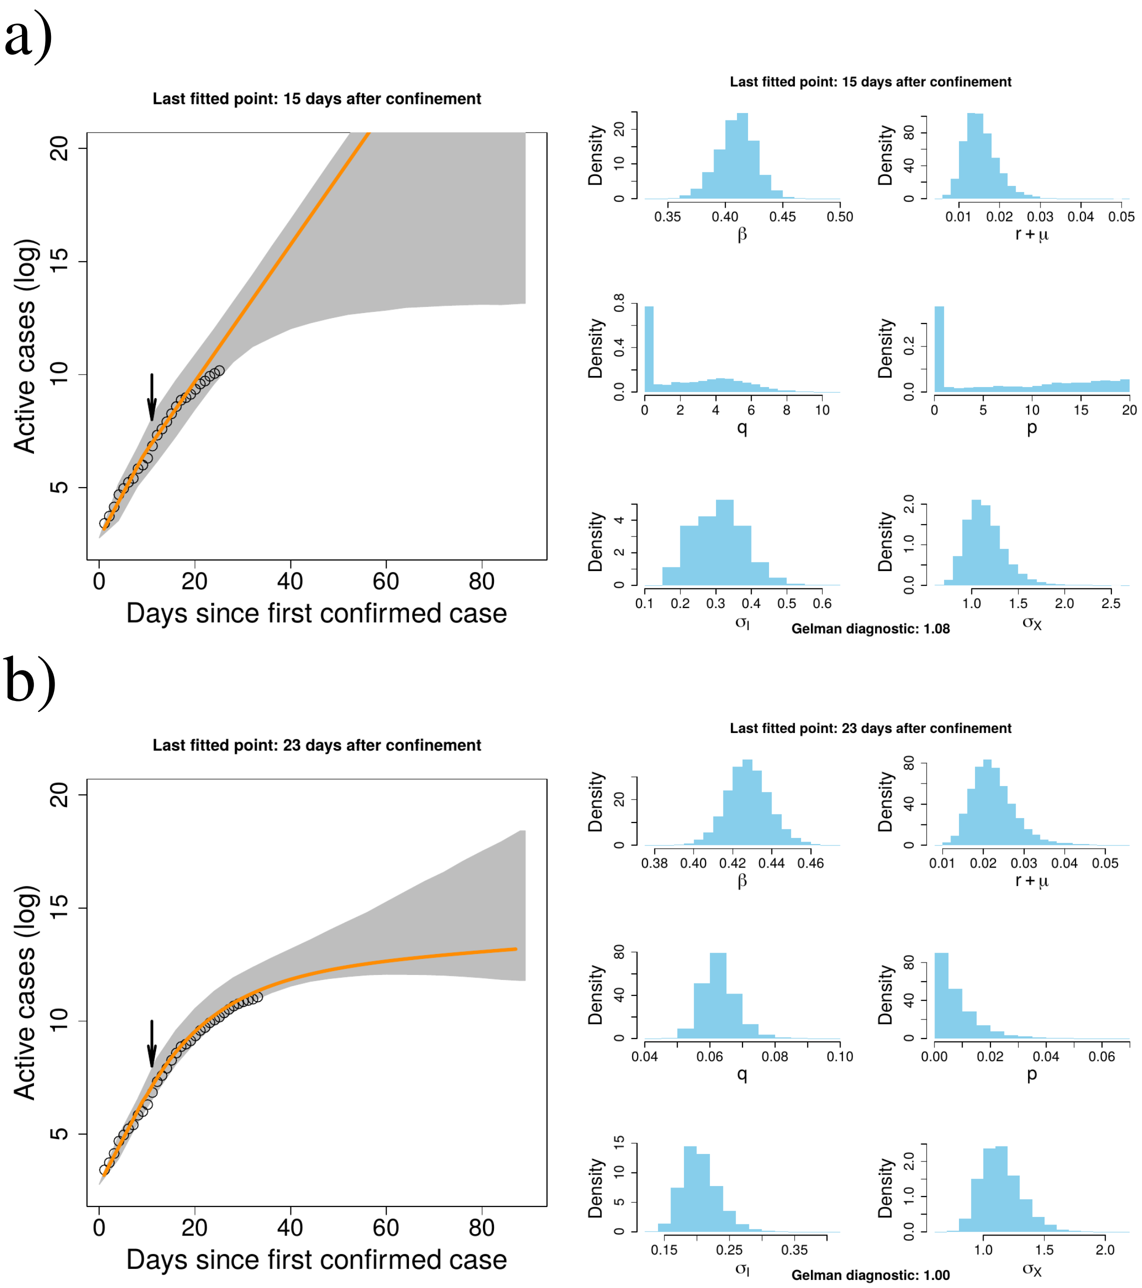


Figure S7: Median estimate with a 95% posterior predictive and posterior density using empirical data. a) Data up to 15 days after confinement. Left: Median and 95% posterior predictive. Right: Posteriors of the parameters learnt from that data. Note that both $p$ and $q$ exhibit multimodality allowing for two possible outcomes: controlled epidemic and exponential growth. b) Panels as in a) but up to 23 days after confinement. After a sufficiently long track of data after confinement, all parameters converge, although the variability still shows that the probability of having inhibited propagation is not 100%, as discussed in the main text.

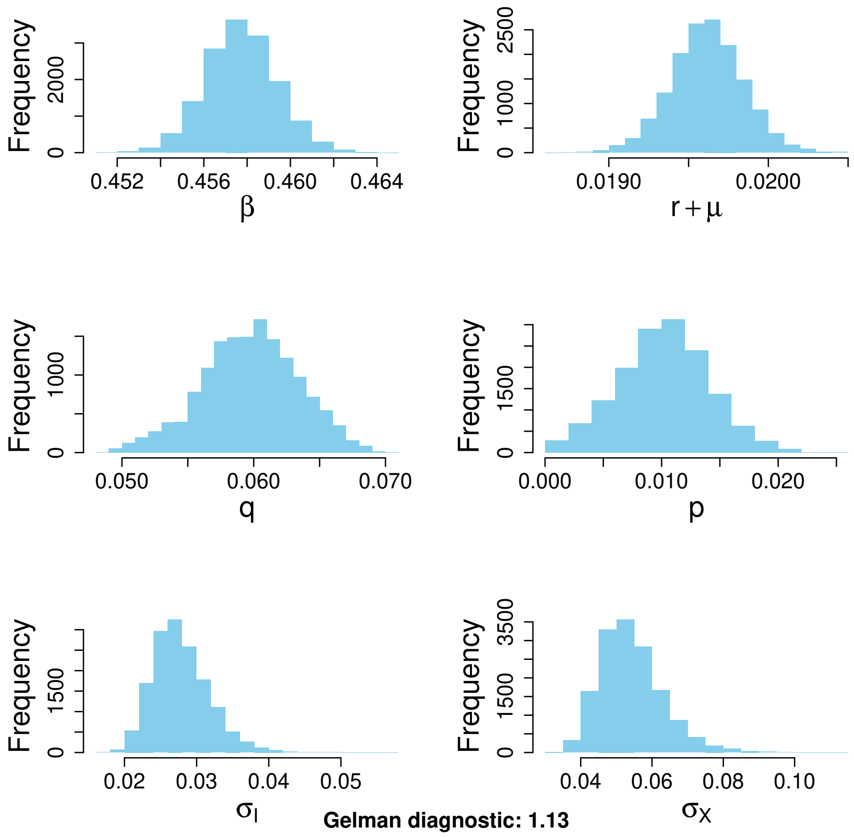


Figure S8: Parameter posteriors for the fit in Fig. 4 in the main text. The multivariate potential reduction factor is 1.13. Values close to 1 mean that different initial conditions in the Monte-Carlo Markov Chain algorithm converge with high accuracy and the fitted posteriors are reliable (see Ref. [2] for details).

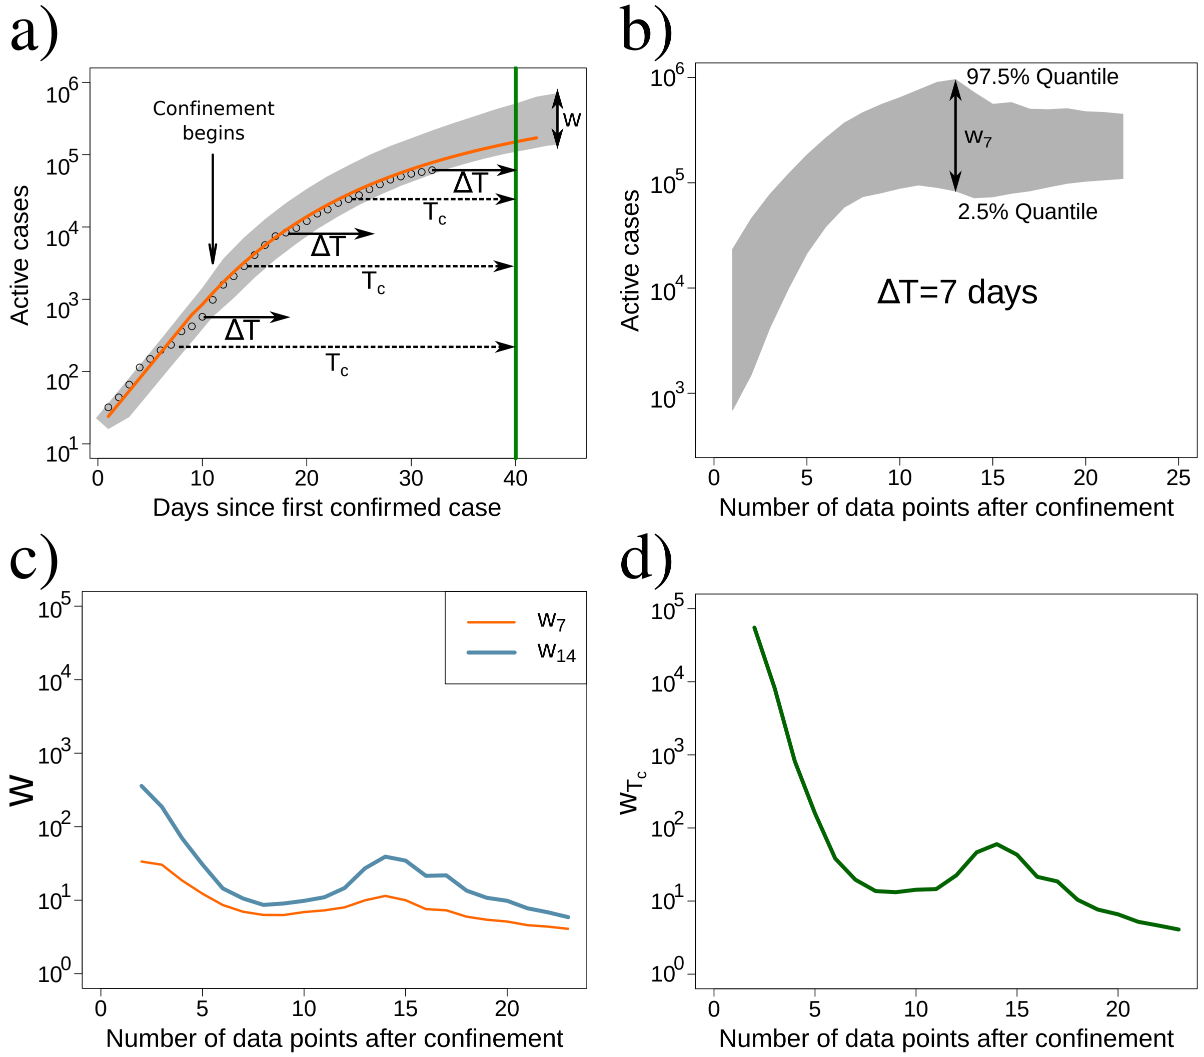


Figure S9: The uncertainty of forecasts does not decrease monotonously with the amount of empirical data. a) Illustration of the fit to empirical data up to March 29th. The beginning of confinement is indicated, as well as the width of the 95% posterior, $w = \log(\text{active } 97.5\%) - \log(\text{active } 2.5\%)$. In subsequent panels we show how w varies at a fixed time interval from the present, $\Delta T$, and at a fixed time in the future, $T_c$. (Note that in the latter case the time interval until prediction shortens monotonously as new data points are added.) b) The grey band shows the breadth of the 95% posterior, $w_7$, seven days after the last data point fitted. c) Variation of the breadth of the 95% posterior with the number of data points fitted, 7 days ($w_7$) and 14 days ($w_{14}$) after the present. Notice that these quantities do not always decrease as more data points are added. d) As in c) for a fixed time in the future, $T_c$ = April 18th. Though in this case the time interval diminishes as more data are added, this does not entail a steady improvement of the forecast.

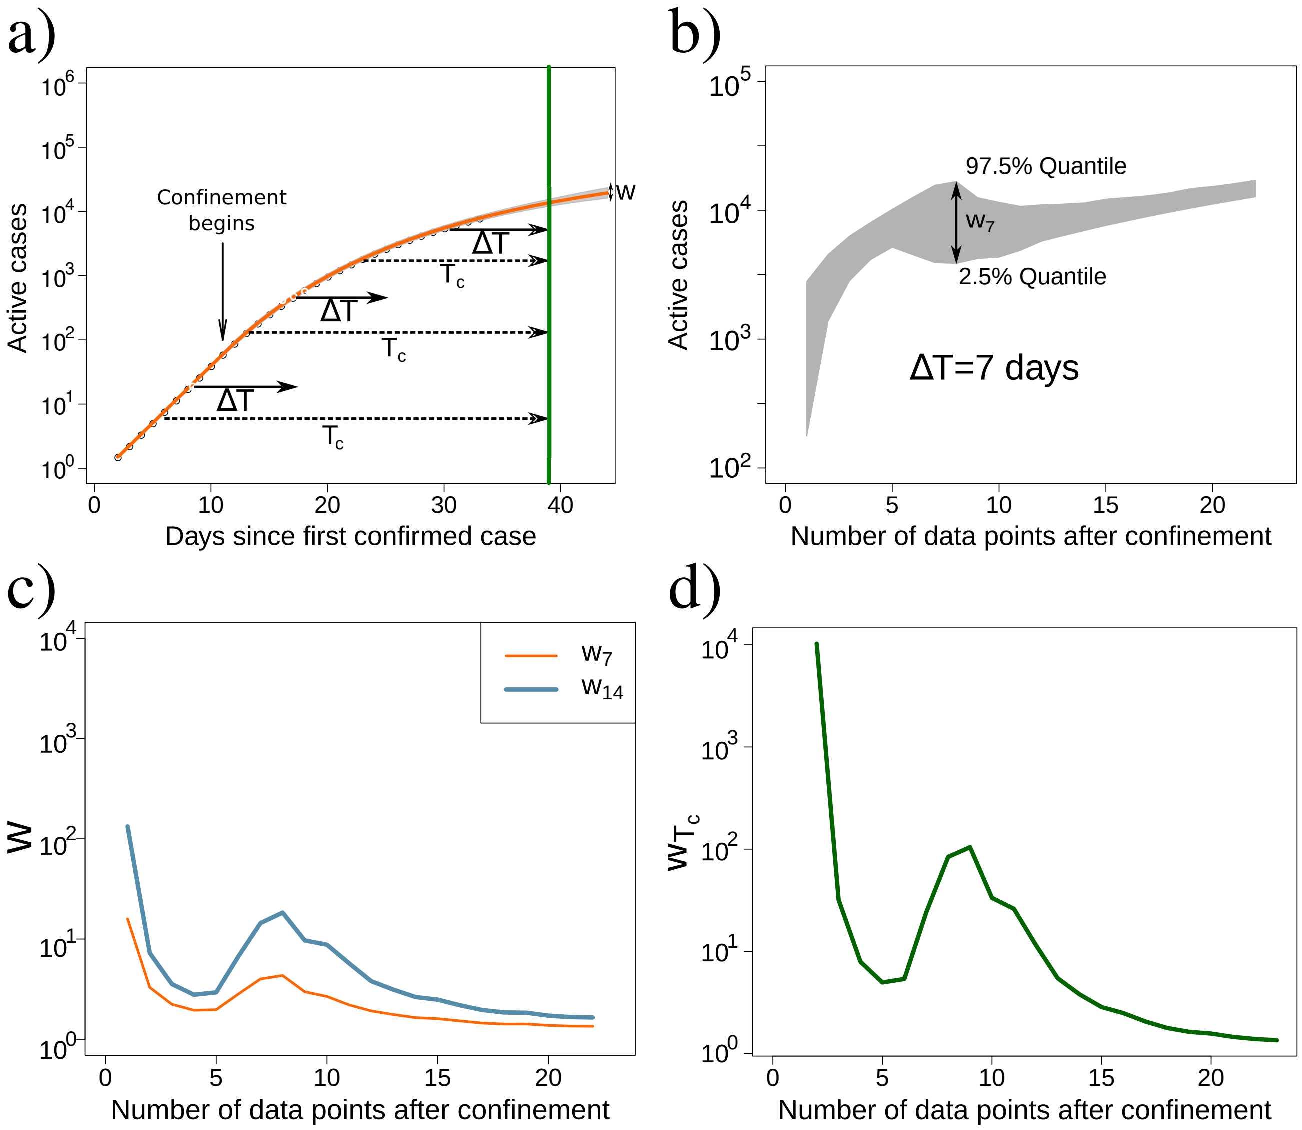


Figure S10: The uncertainty of forecasts does not decrease monotonously with the amount of synthetic data. Panels and symbols are as in the previous figure, but data have been generated through direct simulation of the system described in Figure 1, with parameter values $\beta = 0.425$, $p = 0.007$, $q = 0.062$ and $r + \mu = 0.021$, as in Fig. 4 of the main text. These results, fully consistent with those in Figure S9, show that the non-monotonicity of forecast precision with number of data does not depend on the quality of data, but it is an intrinsic property of the SCIR class of epidemic models.

# D Suitability and limitations of phenomenological models: Gompertz growth curve as example

Besides the use of compartmental models (SIR, SEIR, ...) some authors have proposed the use of phenomenological models, such as the logistic [3] or Gompertz growth curves [4] to reproduce COVID-19 data. For the latter class of models, the total number of confirmed cases, $T(t)$, is described by a universal curve of the form,

$$T(t) = K \exp\left(-\exp(-c(t-t_0))\right),$$

where $t_0$ denotes the beginning of the epidemic. A more handy way to understand the Gompertz curve is by means of the reparametrization

$$T(t) = K \exp\left(-\frac{b}{c}\exp(-ct)\right). \tag{S4}$$

The shape of the curve is an asymmetric sigmoid, where $K = \lim_{t\to\infty} T(t)$ is the steady state. For short times, it is straightforward to see that

$$\log T(t) = \log K - \frac{b}{c} + bt + \cdots, \tag{S5}$$

hence the Gompertz curve provides a simple explanation of the ubiquitous initial exponential growth, $T(t) \sim e^{bt}$. The parameter $c^{-1}$ quantifies the time-scale of viral propagation in the population.

The Gompertz curve has an inflection point (corresponding to the *peak* of the epidemic, $t_{\text{peak}}$) that can be found as the time where

$$\frac{d^2T}{dt^2} = 0 \quad \Rightarrow \quad t_{\text{peak}} = -\frac{\log\left(\frac{c}{b}\right)}{c}.$$

One limitation of these growth curves is that they always predict saturation in the long run. This fact renders the Gompertz curve a suitable phenomenological description of epidemics that spread until herd immunity is reached, but this represents a strong limitation when epidemics are controlled through non-pharmaceutical measures (such as confinement), because these measures not always manage to control the epidemic. This is an important difference with respect to the SCIR model that we use in our article, where the asymptotic behavior can be a growing exponential if control fails.

The growth curve has three free parameters ($b$, $c$ and $K$) that, once estimated, provide information about the early doubling time, the location of the peak and the total number of infected at the end of the epidemic. However, these parameters cannot be estimated freely as they are bounded by the empirical evidence. In particular, $K$ cannot be larger than the total population and, as we discussed in the main text, doubling times larger than 1 are reported in all cases so $b < \log(2)/1\,\text{day}^{-1}$.

In Fig. S11 we show different fits of the empirical data for Spain to the Gompertz growth curve. In particular, in columns a), c) and e) we use the informative prior

$$b \sim \text{Uniform}(0, \log(2))$$

and in columns b), d) and f), the non-informative prior

$$b \sim \text{Uniform}(0, 10).$$

Note how the use of a realistic prior provides less confident predictions (95% posterior interval). In all cases, the model fails to predict either the location of the peak or the end of the epidemic (and, of course, subsequent epidemic bursts). This is due to the lack of flexibility of the model to accommodate with only three parameters all the information about the initial growth rate, the inflection point, the decay into the steady state, etc. This result is striking, because in panels c)–f) the data used to fit the curves include the real (observed) epidemic peak.

It is worth mentioning that (S3) generalizes both the basic SIR model and the Gompertz growth.

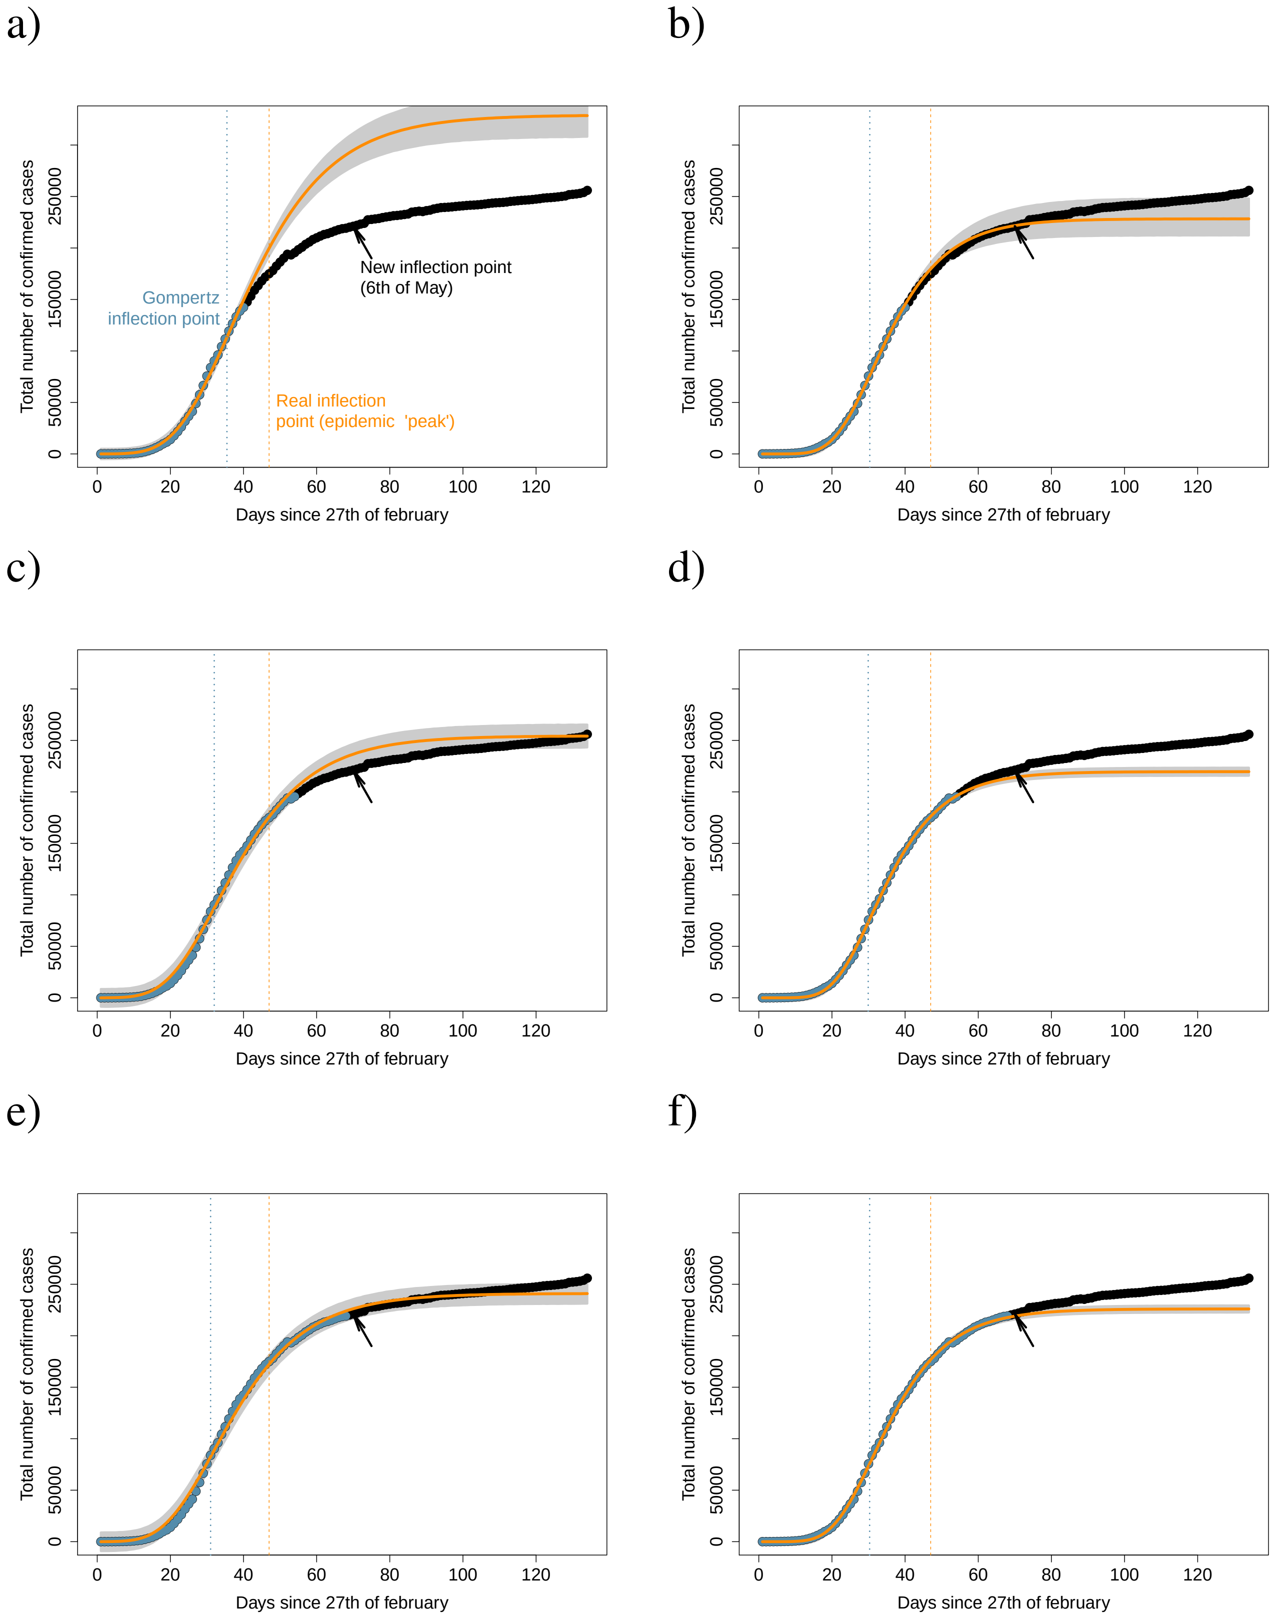


Figure S11: The Gompertz curve neither can model the effect of confinement nor predict the peak and end of the epidemic. Black circles show the total number of confirmed cases (real data for Spain, see Sec. B. The data used to fit the parameters in each panel are shown in blue. The shaded area represent the 95% posterior prediction. a) Informative prior: 7 days before the real peak. b) Non-informative prior: 7 days before the real peak. c) Informative prior: 7 days after the real peak. d) Non-informative prior: 7 days after the real peak. e) Informative prior: 21 days after the real peak. f) Non-informative prior: 21 days after the real peak.

# References

[1] Marina Pollán, Beatriz Pérez-Gómez, Roberto Pastor-Barriuso, Jesús Oteo, Miguel A Hernán, Mayte Pérez-Olmeda, Jose L Sanmartín, Aurora Fernández-García, Israel Cruz, Nerea Fernández de Larrea, et al. Prevalence of SARS-CoV-2 in Spain (ENE-COVID): a nationwide, population-based seroepidemiological study. *The Lancet*, 2020.

[2] Andrew Gelman, Donald B Rubin, et al. Inference from iterative simulation using multiple sequences. *Statistical science*, 7(4):457–472, 1992.

[3] Ke Wu, Didier Darcet, Qian Wang, and Didier Sornette. Generalized logistic growth modeling of the COVID-19 outbreak in 29 provinces in China and in the rest of the world. 2020. arXiv:2003.05681.

[4] Michael Levitt, Andrea Scaiewicz, and Francesco Zonta. Predicting the trajectory of any COVID19 epidemic from the best straight line. *medRxiv*, 2020.
